# Supplementary material for: Electrostatic trapping of N$_2$ molecules in high Rydberg states
Source: arXiv:2403.12315 source file (2024-03-18)
Supplement: Supplementary file 1 [file Supplemental_Material_N2_trapping.pdf]

# Supplemental Material for 'Electrostatic trapping $N_2$ molecules in high Rydberg states'

M. H. Rayment and S. D. Hogan
*Department of Physics and Astronomy, University College London, Gower Street, London WC1E 6BT, United Kingdom*
(Dated: January 15, 2024)

To aid in the interpretation of the changes in the effective trap decay time constants with $n$ for $N_2$ in Fig. 4(c) of the main article, additional experiments were performed with helium (He) atoms in singlet Rydberg states. These were carried out in the same apparatus and allowed for directly comparable studies of trap decay dynamics in a system devoid of intramolecular charge-multipole interactions, and non-radiative decay processes. In this work, pulsed supersonic beams of He in the metastable $1s2s\,^1S_0$ level were generated in a dc electric discharge at the exit of the pulsed valve [S1]. An electrostatic filter was installed on the axis of propagation of the beam after the skimmer to remove charged particles generated in the discharge. After entering the decelerator structure, the atoms were photoexcited to Rydberg states with $1snp\,^1P_1$ character in a single-photon transition at wavelengths of $\sim 313$ nm. The singlet Rydberg states in He were chosen for this work because the singlet-p levels have small quantum defects of $\delta_{n\mathrm{p}} = -0.0121$, which allow for population transfer into $\ell$-mixed Rydberg-Stark states close to the time of laser photoexcitation in a similar way to that which occurs in the experiments with $N_2$ in the main article.

After photoexcitation the Rydberg He atoms were decelerated from an initial speed of $v_i = 2000\ \mathrm{m\,s^{-1}}$ to rest in the laboratory-fixed frame of reference in a time of $\sim 100\ \mu$s, with the decelerator operated in an identical way to that for $N_2$. The effective decay time constants of the atoms from the electrostatic traps were determined using the same fitting procedure as for $N_2$. These trap decay time constants, for Rydberg states with values of $n$ between 34 and 48 are shown in Fig. 1. They range from 300 $\mu$s to 500 $\mu$s and generally increase as the value of $n$ increases. The smaller values of $\tau^*$, than those measured for $N_2$, reflect the lower-$|m_\ell|$ character of the atomic Rydberg states prepared, and that could be trapped, in these experiments.

As in the case of $N_2$, the effective trap decay time constants determined for He do not scale with $\sim n^4$ as might be expected for individual $\ell$-mixed Rydberg-Stark states. The observed trend, that the increase in the value of $\tau^*$ with $n$ becomes less pronounced at higher values of $n$, is however consistent with the preparation of atoms in a distribution of Rydberg-Stark states with different values of $m_\ell$. In this situation, because the higher $|m_\ell|$ states decay more slowly than the lower $|m_\ell|$ states, the decay of atoms from the trap is not described well by a single exponential function.

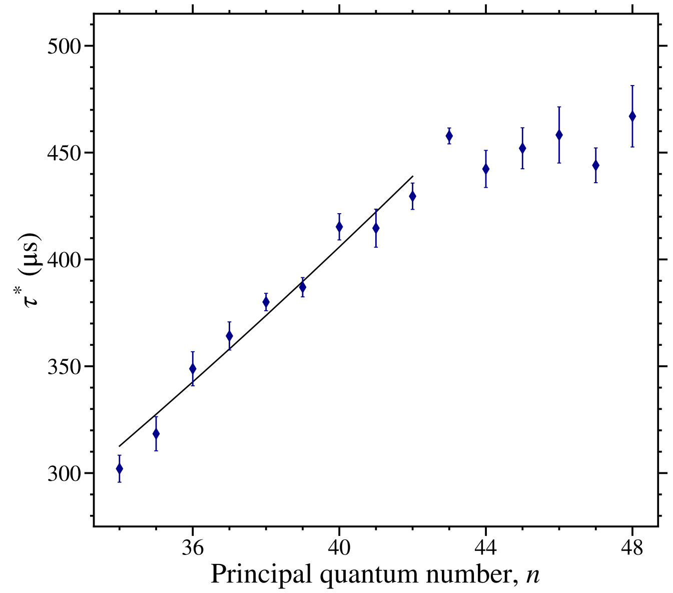


FIG. 1. Effective trap decay time constants, $\tau^*$, for He atoms excited on $1snp\,^1P_1$ resonances to $\ell$-mixed singlet Rydberg-Stark states. The continuous black line represents the function $\tau^* = 1.09\,n^{1.61}\ \mu$s fit to the experimental data.

For lower values of $n$, i.e., $n < 40$ in Fig. 1, the measured trap decay time constants are dominated by contributions from longer-lived $|m_\ell| \geq 2$ Rydberg-Stark states. This is because, even in He, the Stark states with $|m_\ell| \leq 1$ are not sufficiently long-lived to be efficiently decelerated and electrostatically trapped. For higher values of $n$, the values of $\tau^*$ increase more slowly with $n$ because the subset of atoms in $|m_\ell| \leq 1$ Rydberg-Stark states begins to have sufficiently long lifetimes to be trapped, and contribute to the trap decay at early times. The balance between these changes in the distribution of values of $m_\ell$ of the trapped atoms means that the measured decay time constants do not scale in a simple way with $n$. For reference, at the lower values of $n$, between 34 and 42, a least-squares-fit indicates that $\tau^* = 1.09\, n^{1.61\pm0.01}$ $\mu$s as seen from the continuous black curve in Fig. 1. This is similar to the $n$-scaling observed in the corresponding data presented for $N_2$ in Fig. 4(c) of the main article.

[S1] T. Halfmann, J. Koensgen, and K. Bergmann, A source for a high-intensity pulsed beam of metastable helium atoms, Meas. Sci. Technol. **11**, 1510 (2000).
